# Supplementary material for: Jets separated by a large pseudorapidity gap at the Tevatron and at the LHC
Source: arXiv:2206.04965 source file (2022-08-23)

BFKL Cross Section for D0@1.8TeV w/ Exp. gap

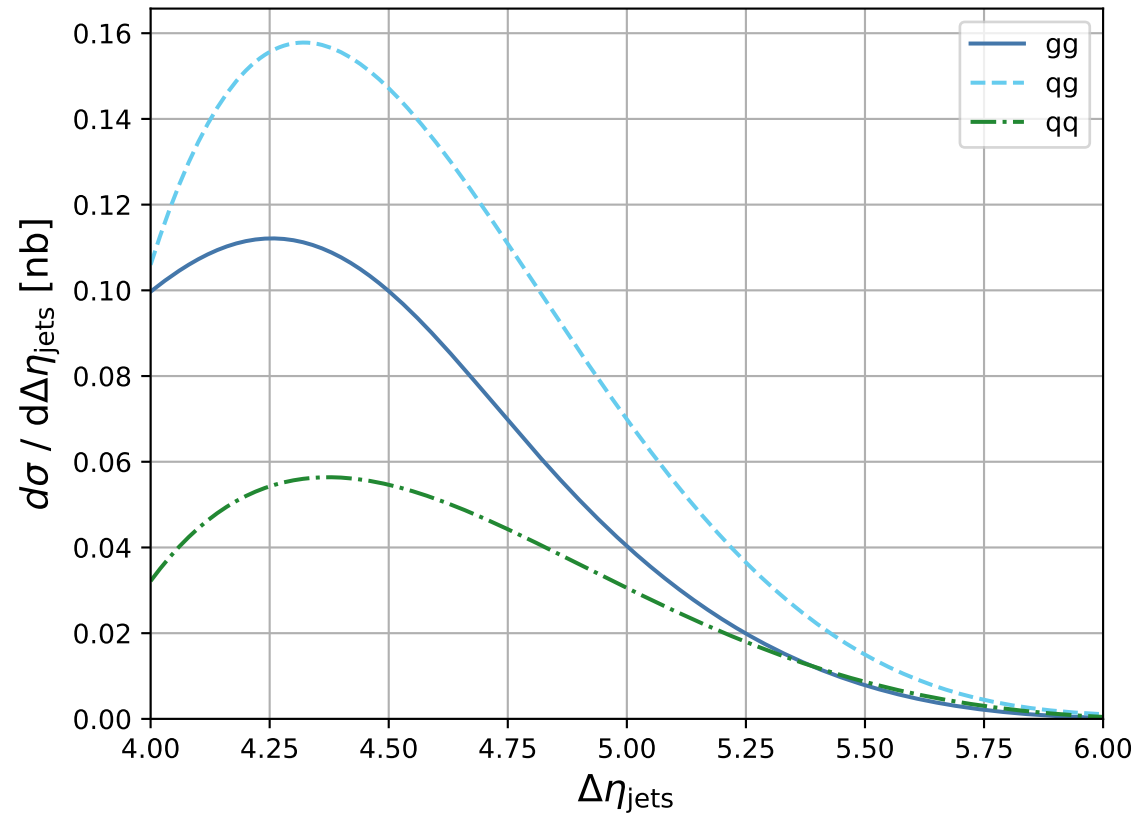

BFKL Cross Section for D0@1.8TeV w/ Strict gap

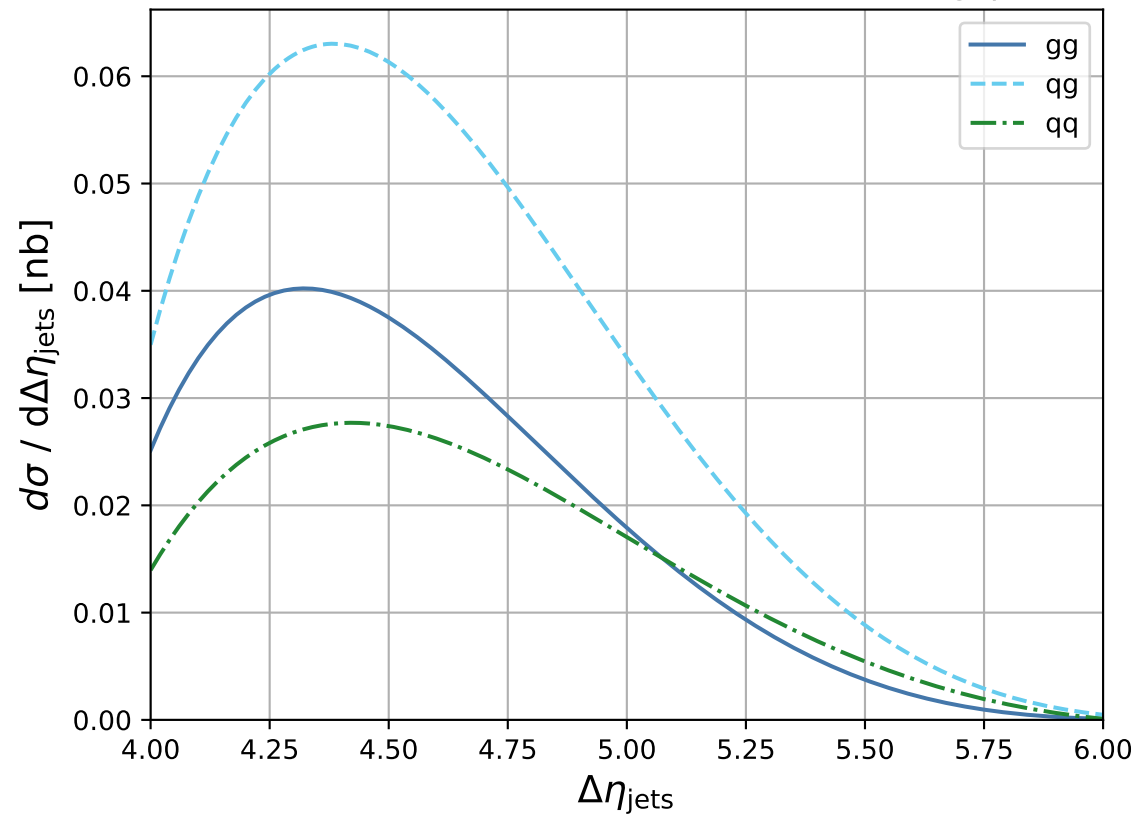

HardQCD Cross Section for D0@1.8TeV

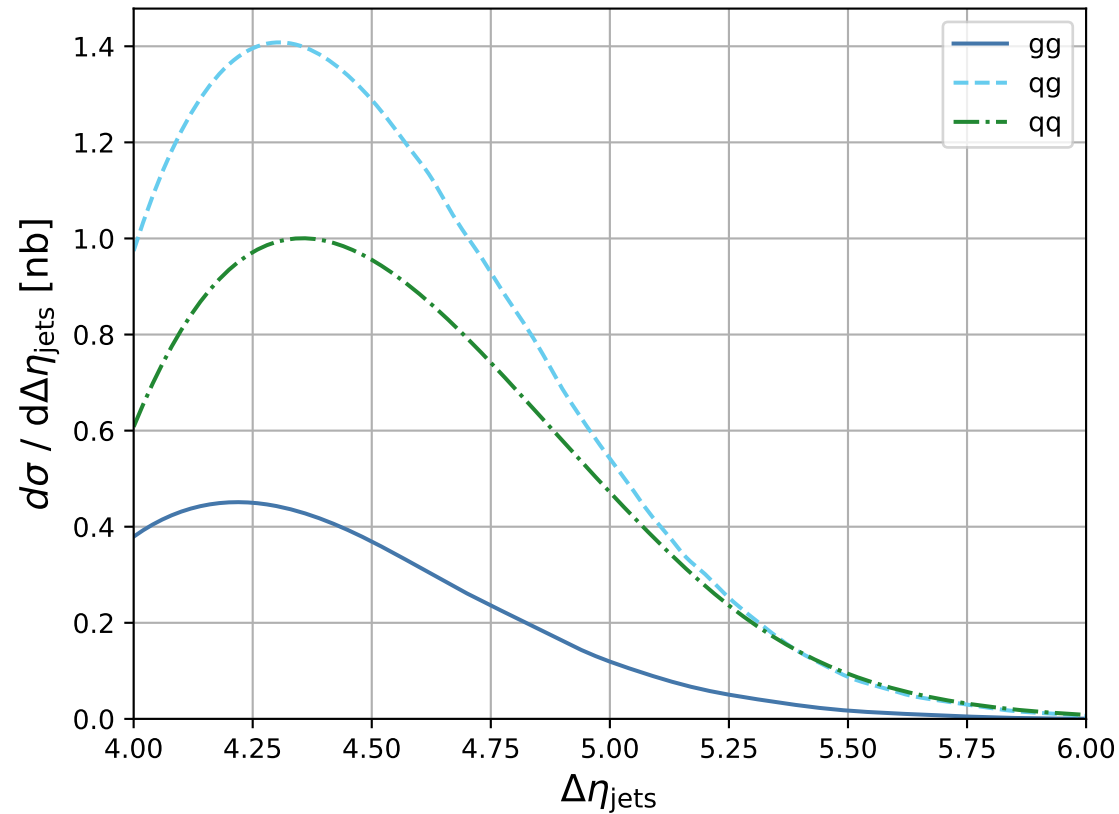

Exp. gap  $f_{\text{CSE}}$  ( $S=0.05$ ) for D0@1.8TeV

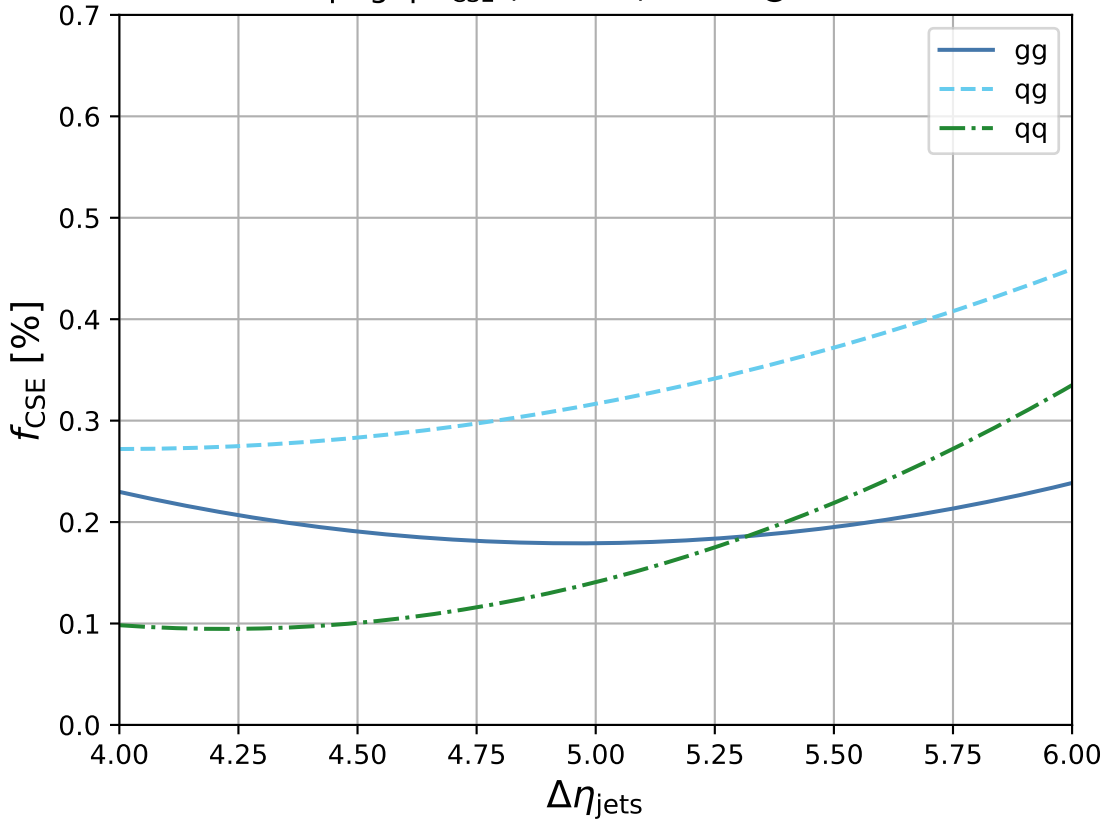

Strict gap  $f_{\text{CSE}} (S=0.1)$  for D0@1.8TeV

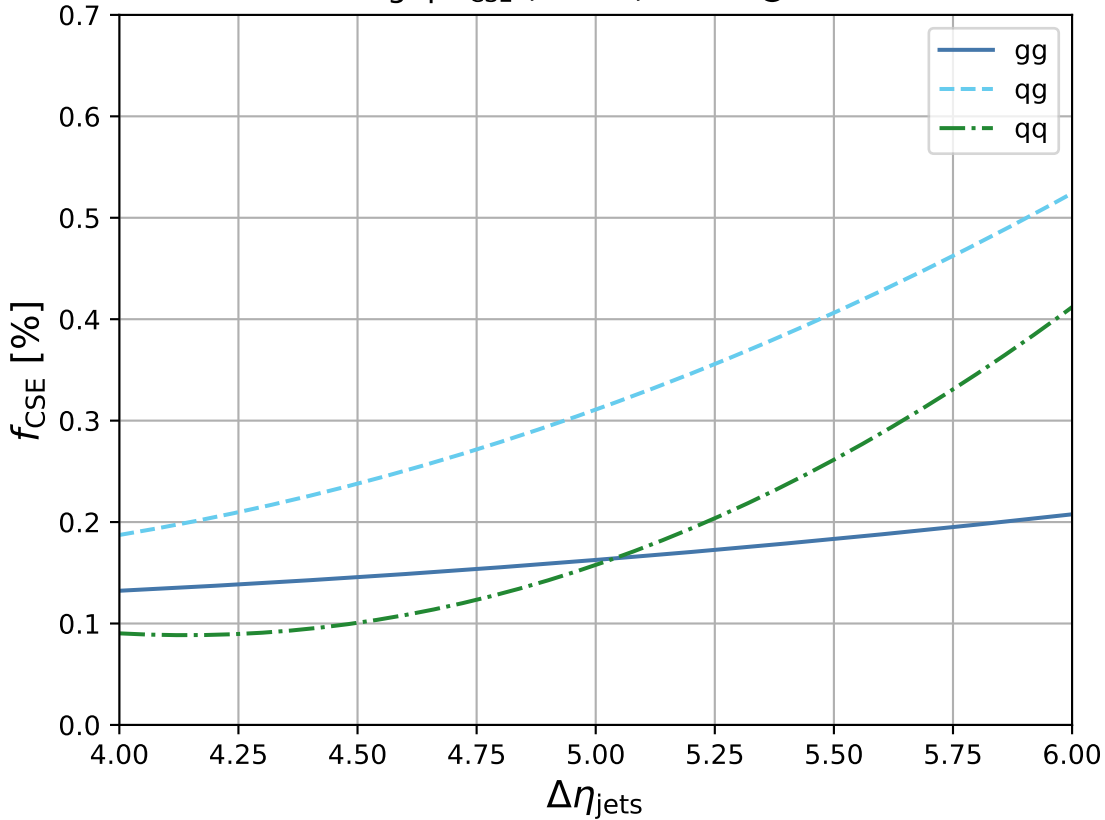

Survival probability using PYTHIA's MPI for D0@1.8TeV

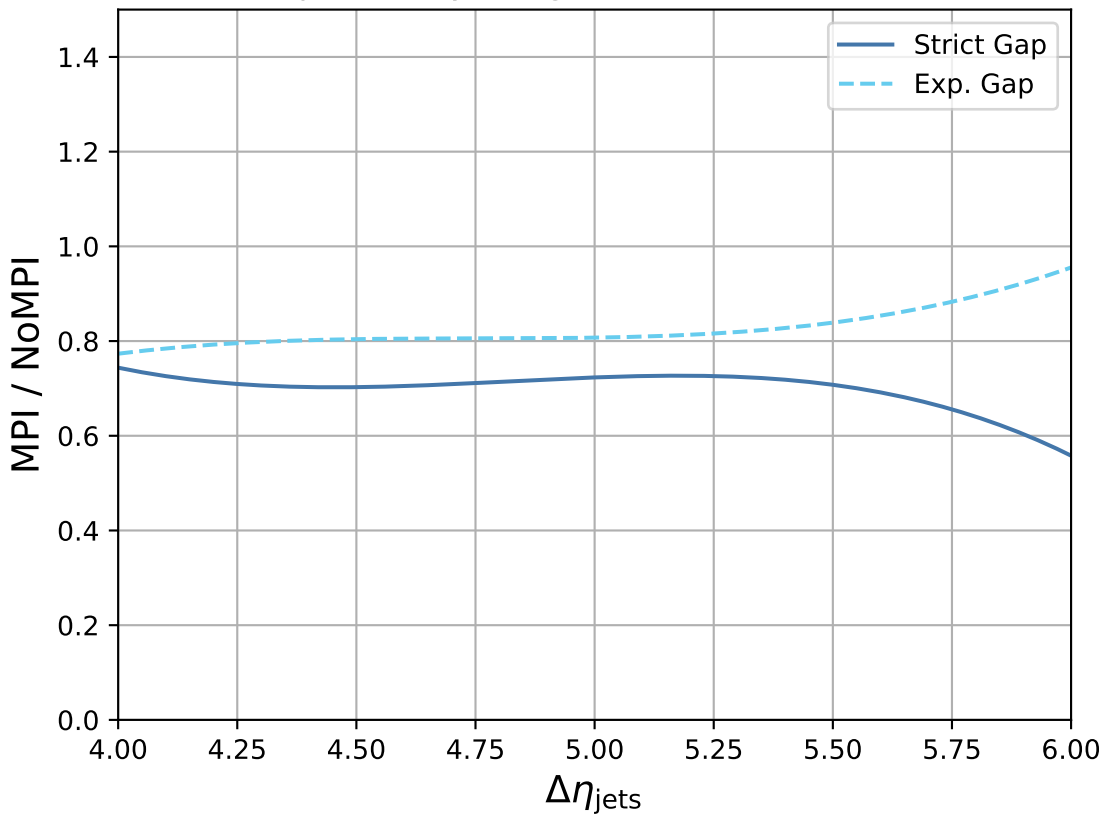

Particle distribution in gap with ISR for D0@1.8TeV

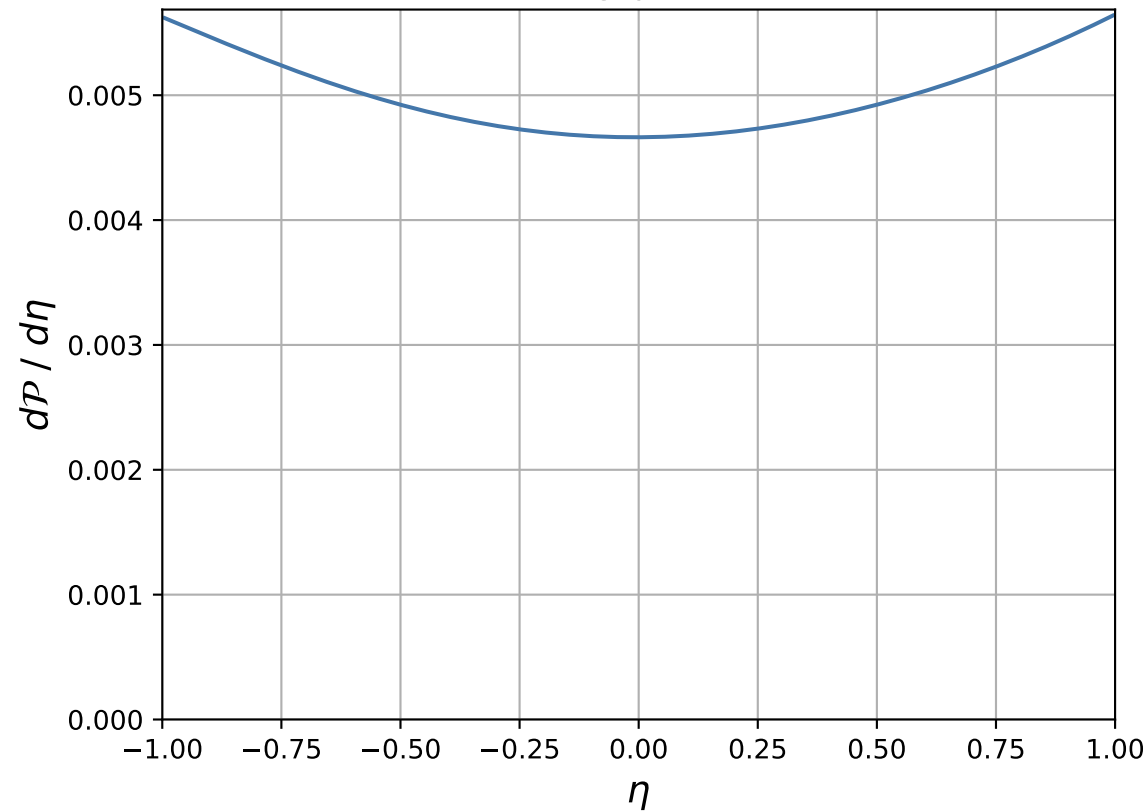

Particle distribution in gap without ISR for D0@1.8TeV

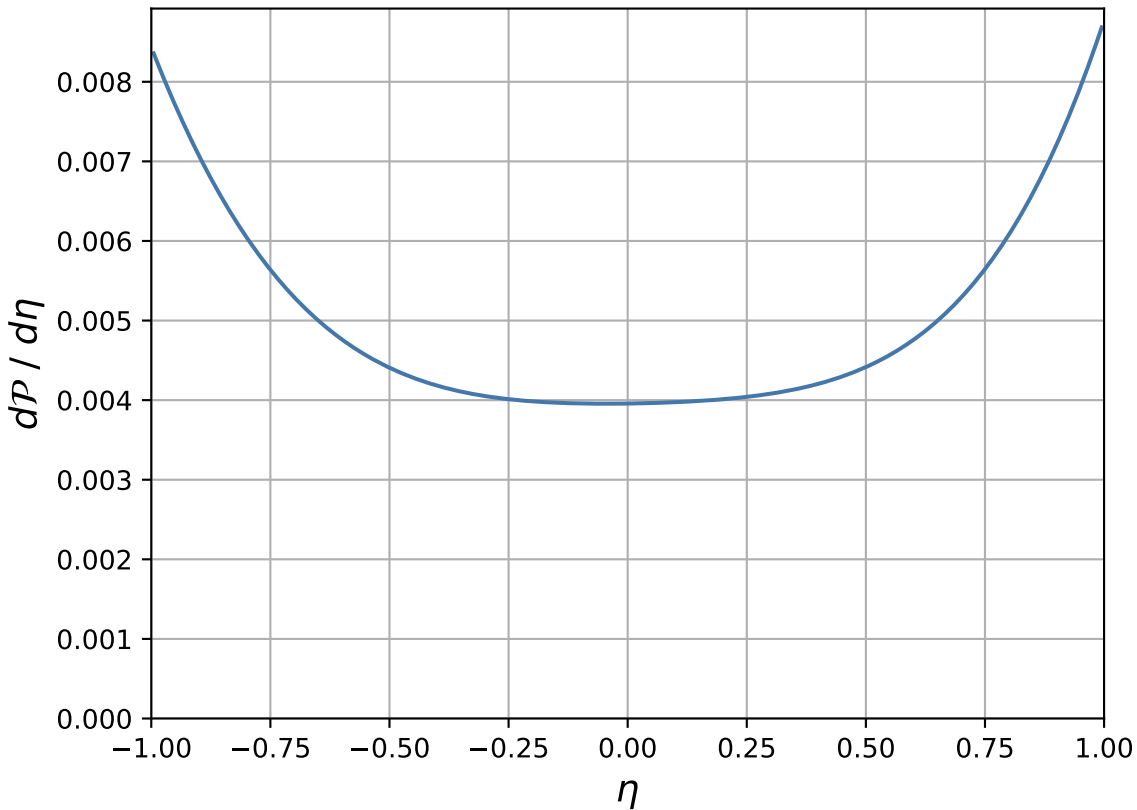



# Tevatron BFKL Strict Gap

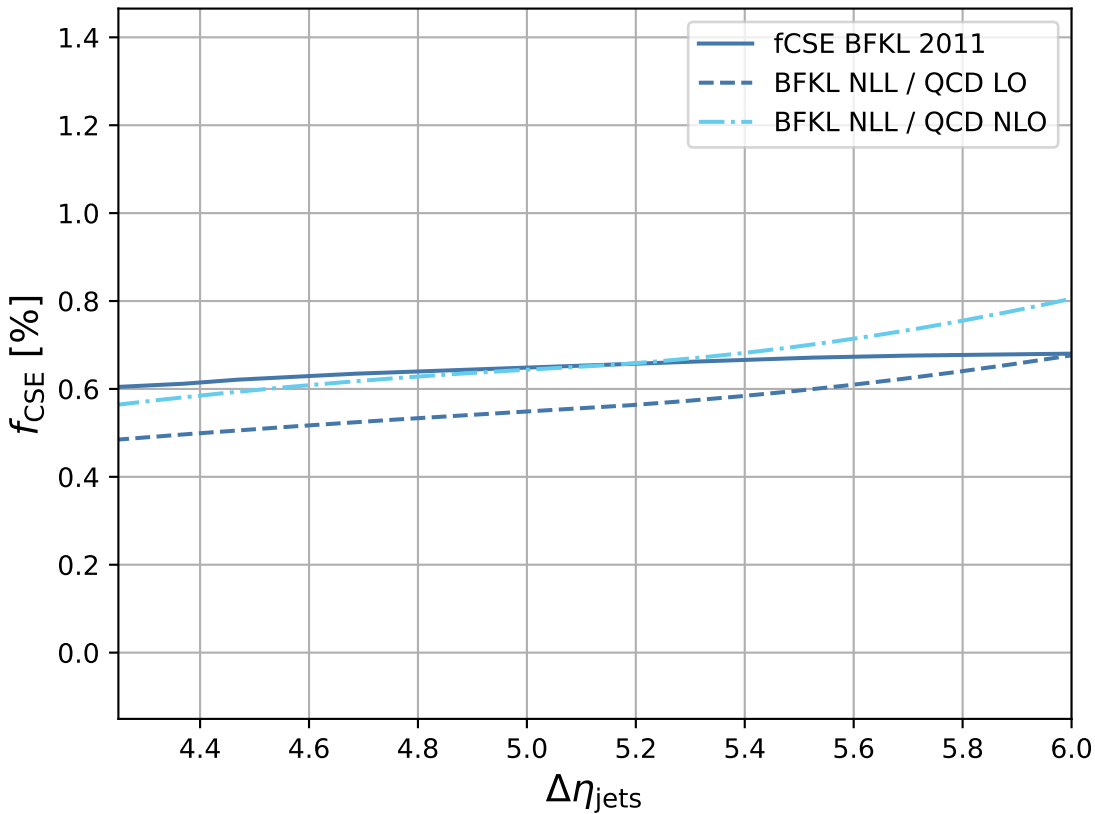

BFKL Strict gap definition for D0@1.8TeV

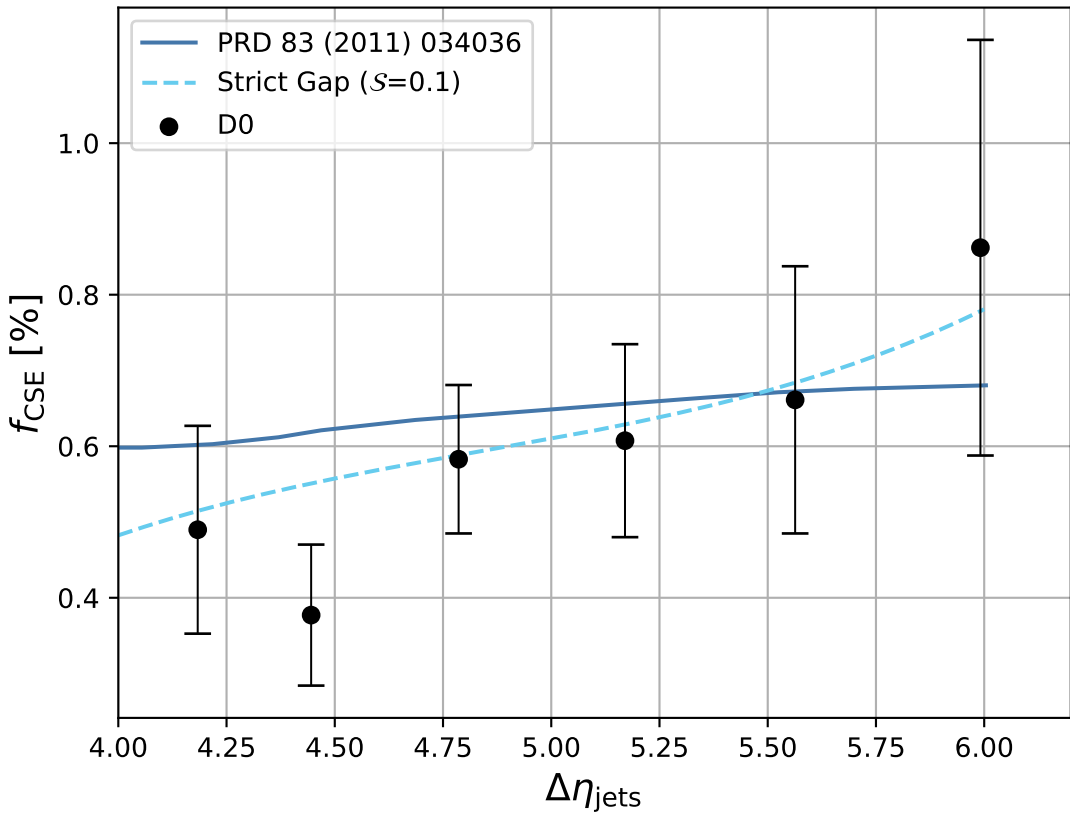

Supplement: Supplementary file 1 [file D0_additional_plots.pdf]
