# Supplementary material for: Jets separated by a large pseudorapidity gap at the Tevatron and at the LHC
Source: arXiv:2206.04965 source file (2022-08-23)

BFKL Cross Section for CMS@13TeV w/ Exp. gap

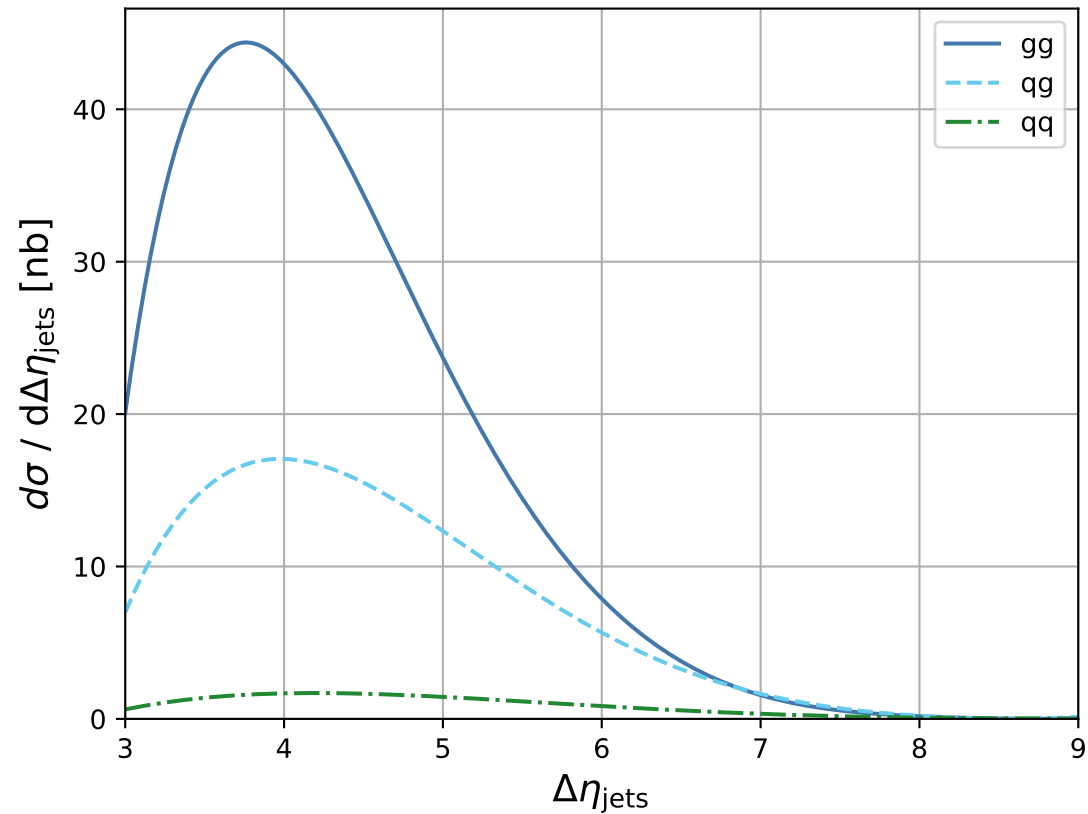

BFKL Cross Section for CMS@13TeV w/ Strict gap

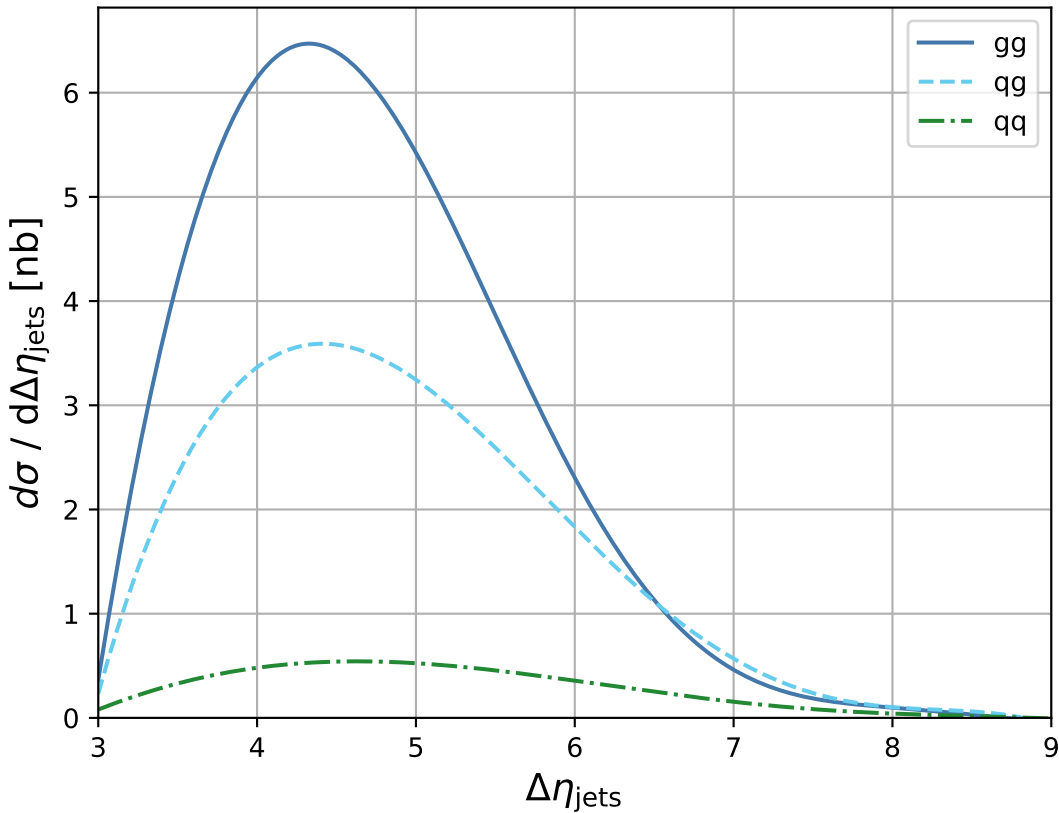

# HardQCD Cross Section for CMS@13TeV

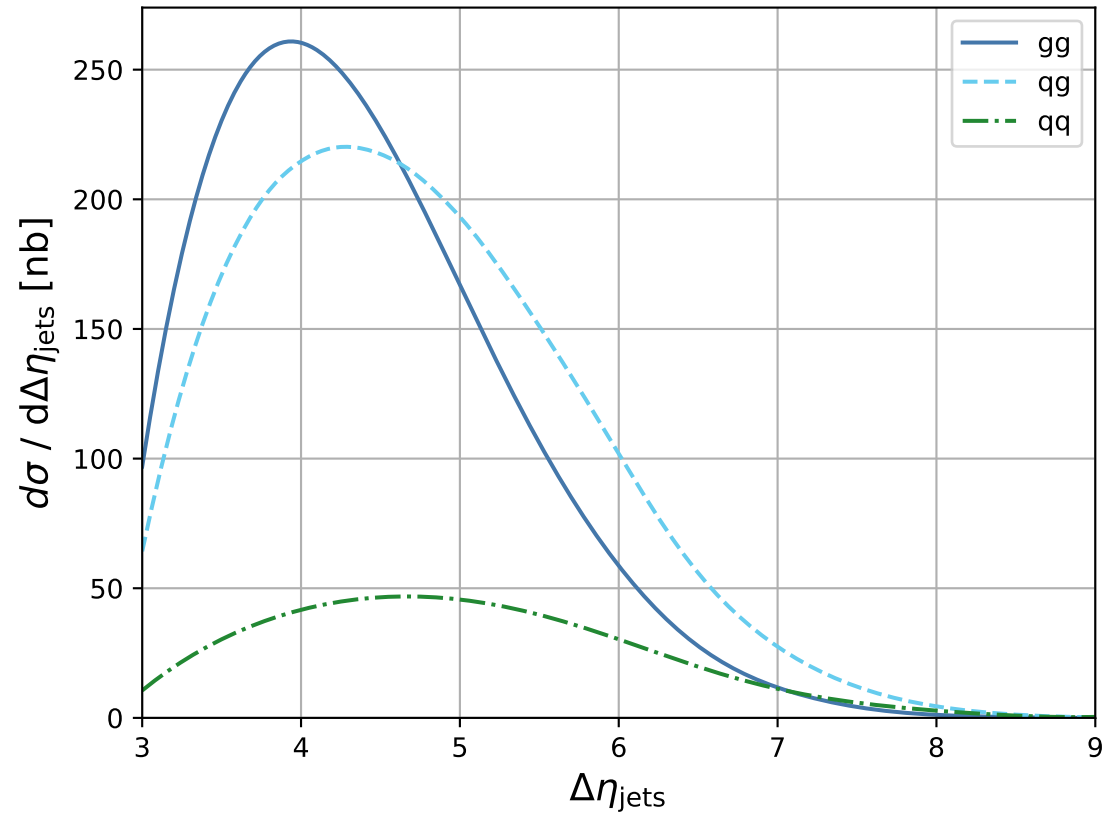

Exp. gap  $f_{\text{CSE}}$  ( $S=0.05$ ) for CMS@13TeV

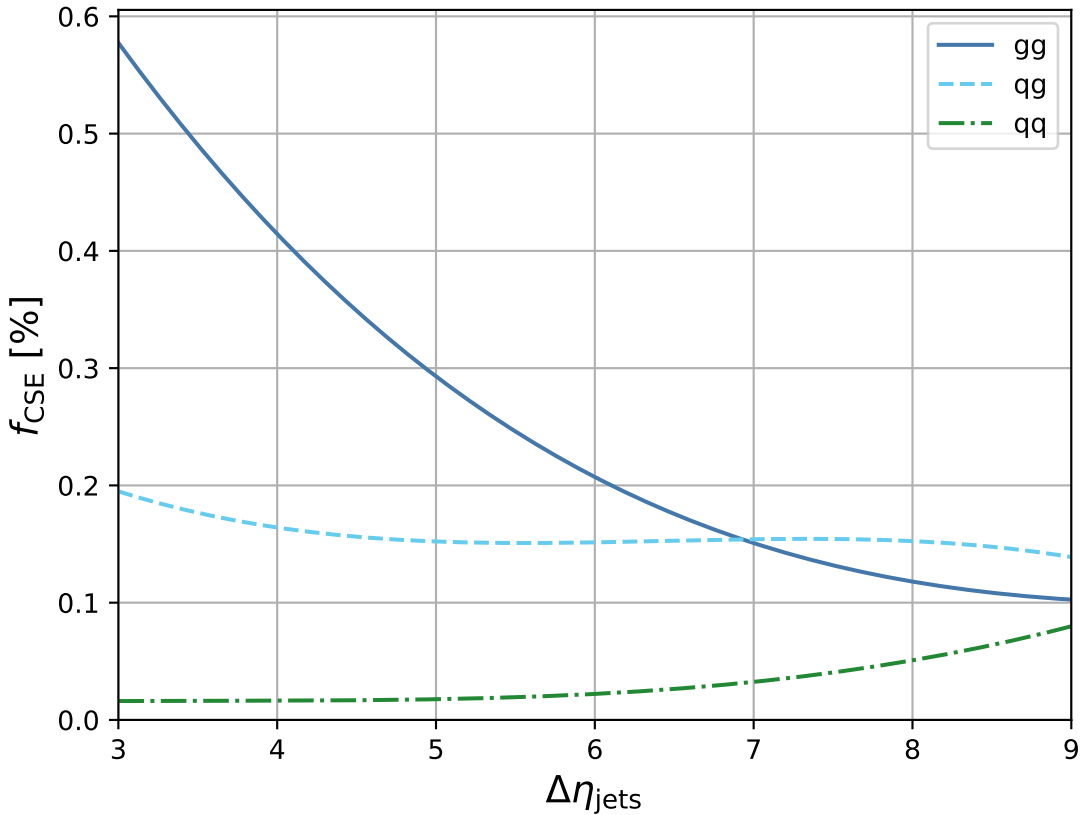

Strict gap  $f_{\text{CSE}}$  ( $s=0.3$ ) for CMS@13TeV

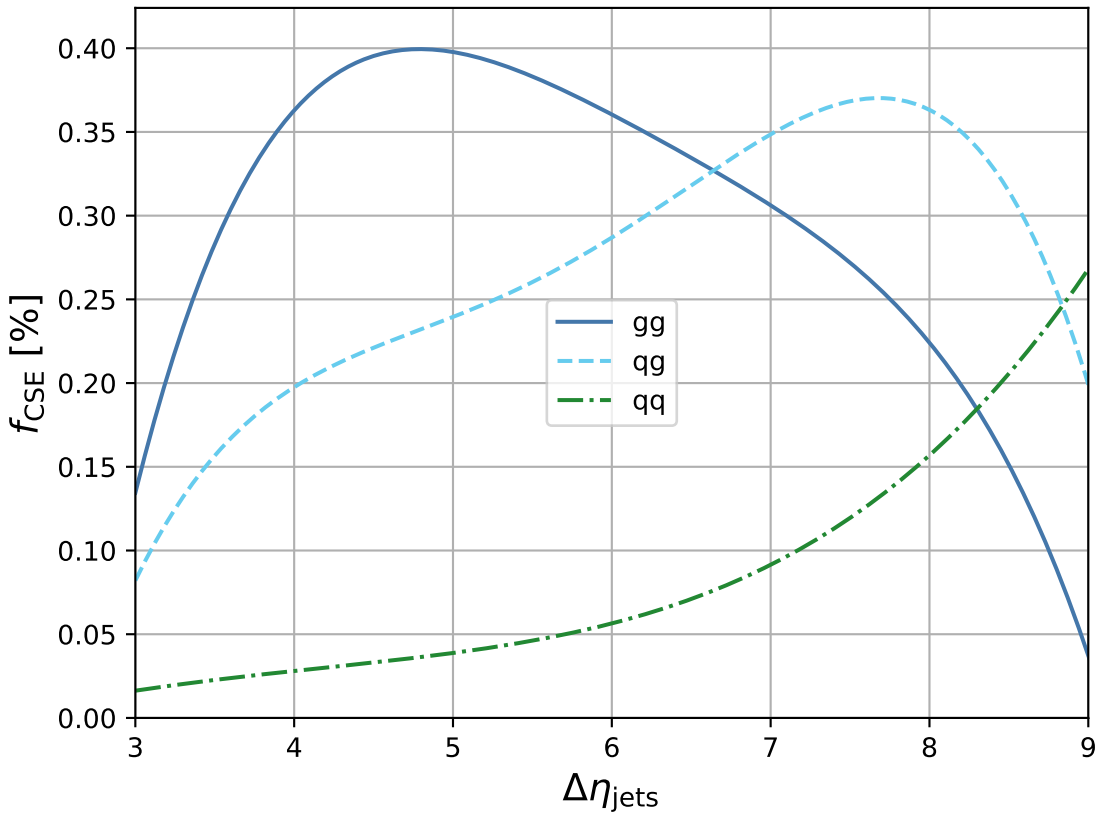

Survival probability using PYTHIA's MPI for CMS@13TeV

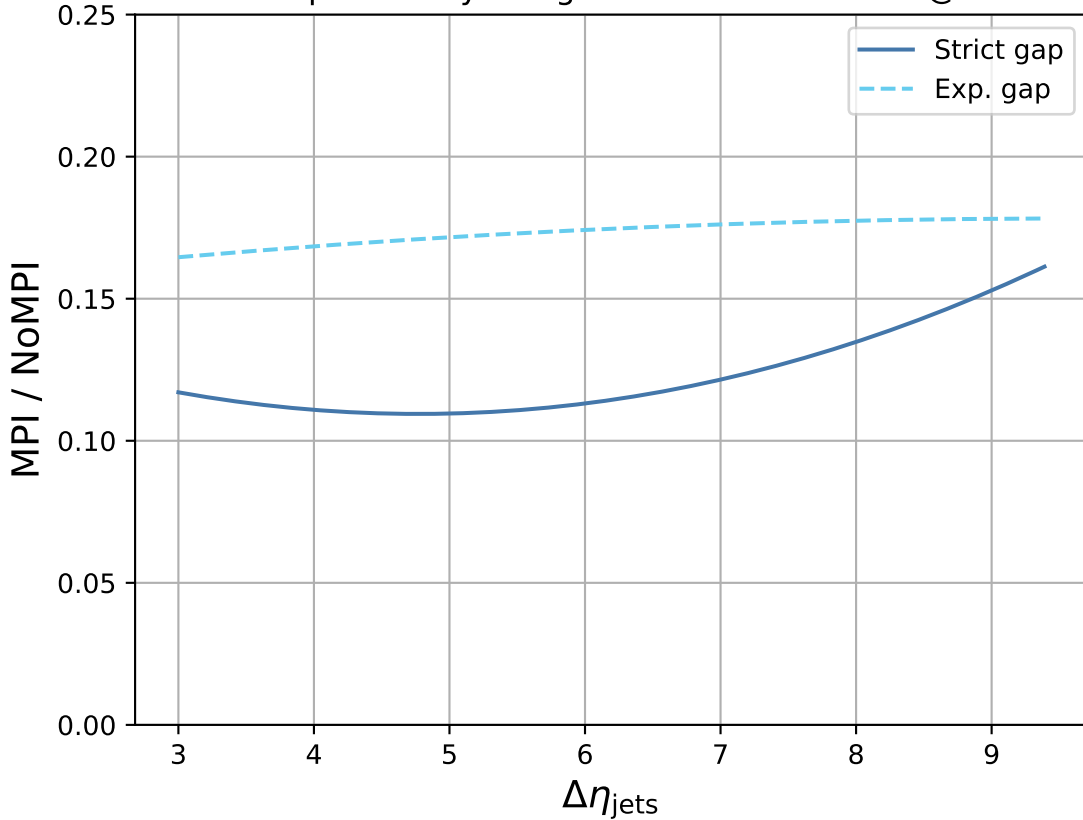

Particle distribution in gap with ISR for CMS@13TeV

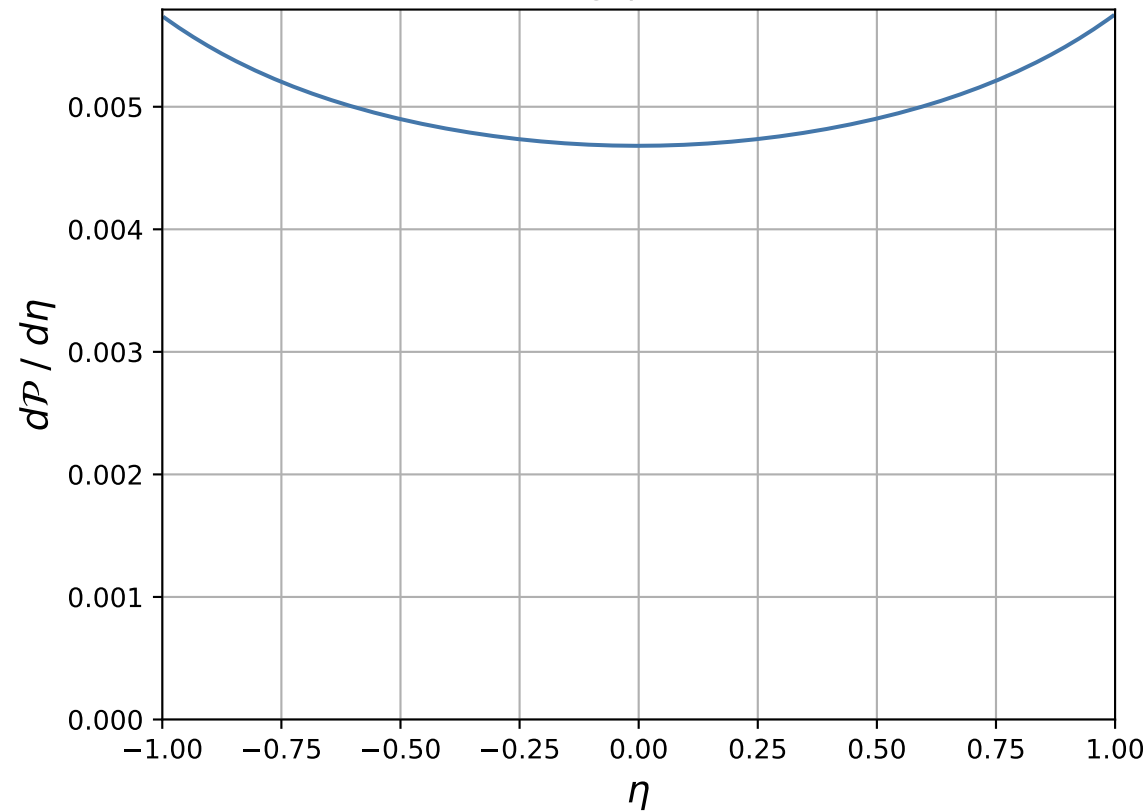

Particle distribution in gap without ISR for CMS@13TeV

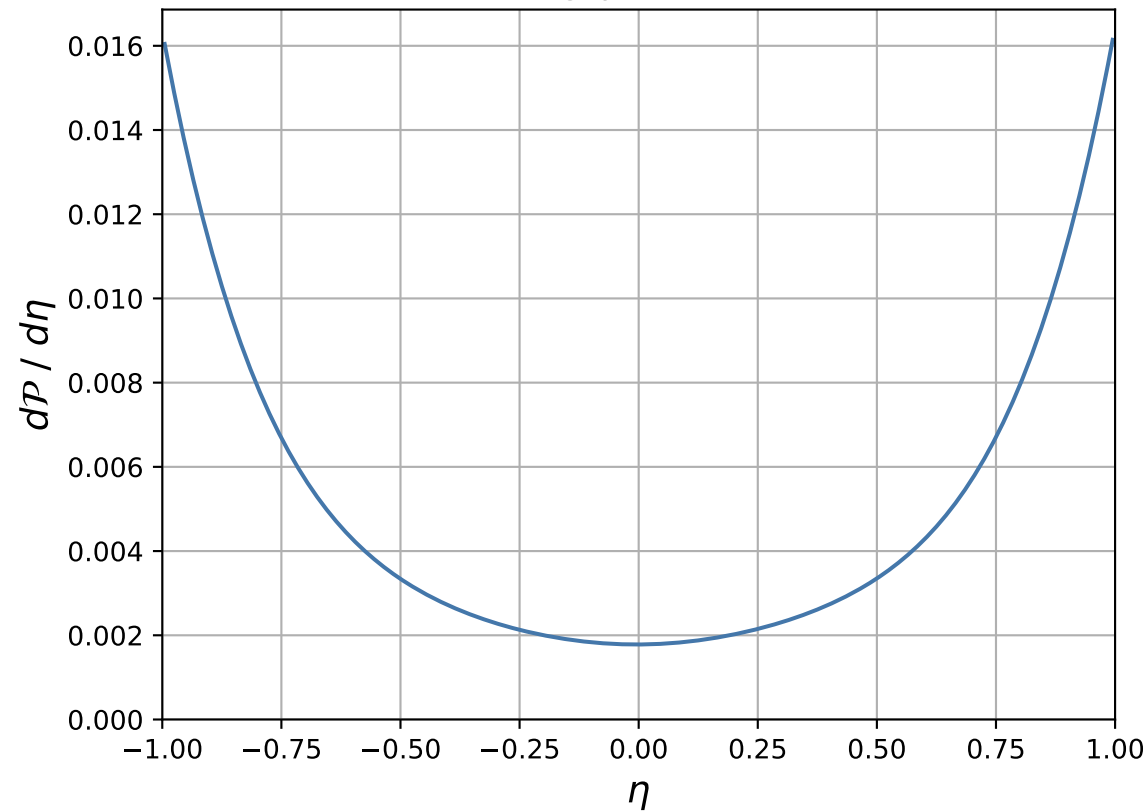



Number of tracks in gap for CMS@13TeV w/ Exp. gap, ISR on

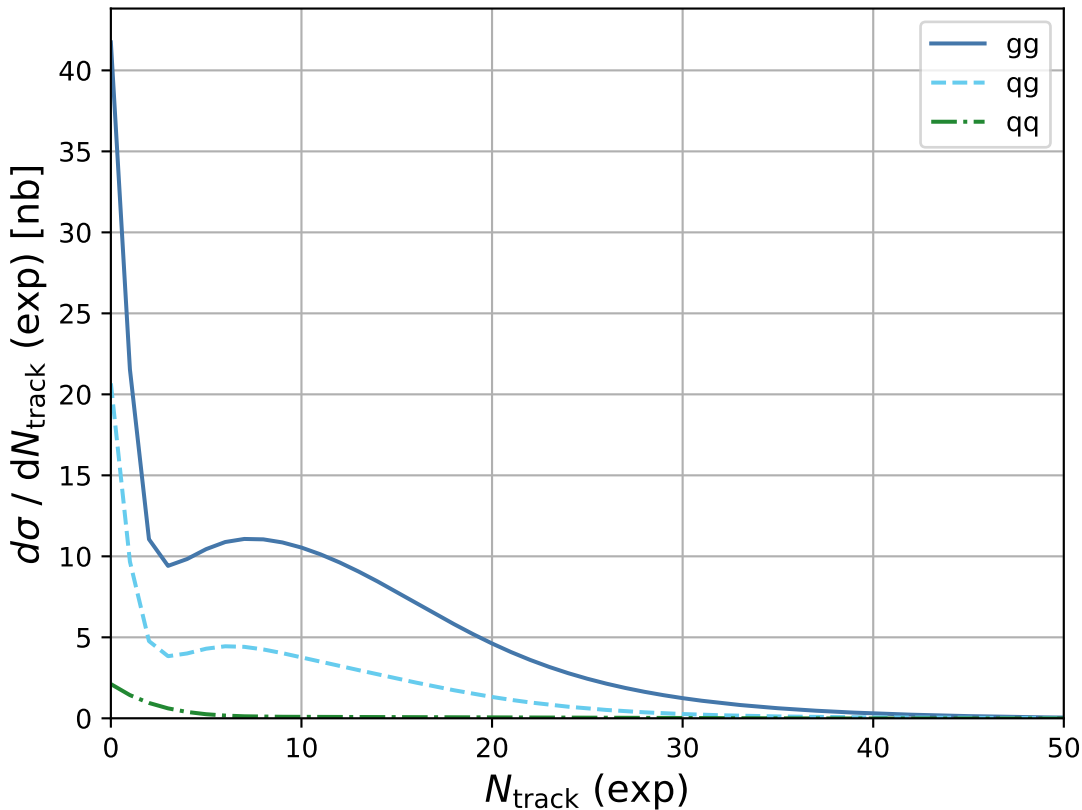

Number of tracks in gap for CMS@13TeV w/ Strict gap, ISR on

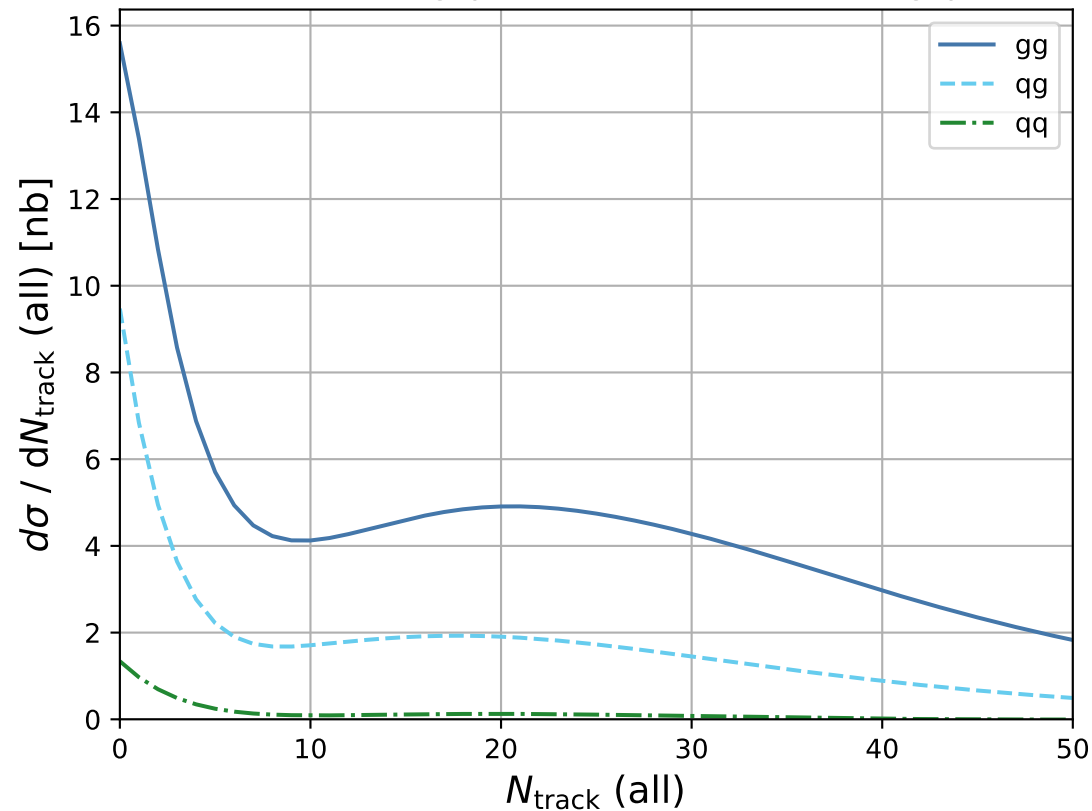

Number of tracks in gap for CMS@13TeV w/ Exp. gap, ISR off

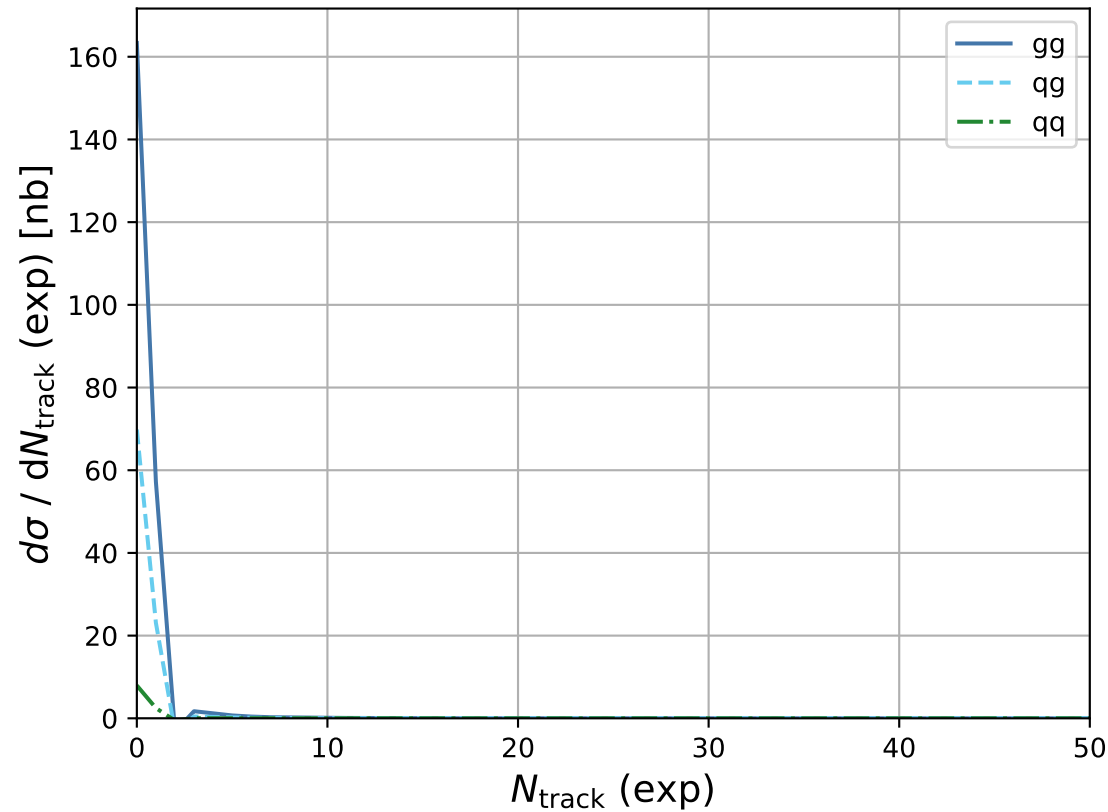

Number of tracks in gap for CMS@13TeV w/ Strict gap, ISR off

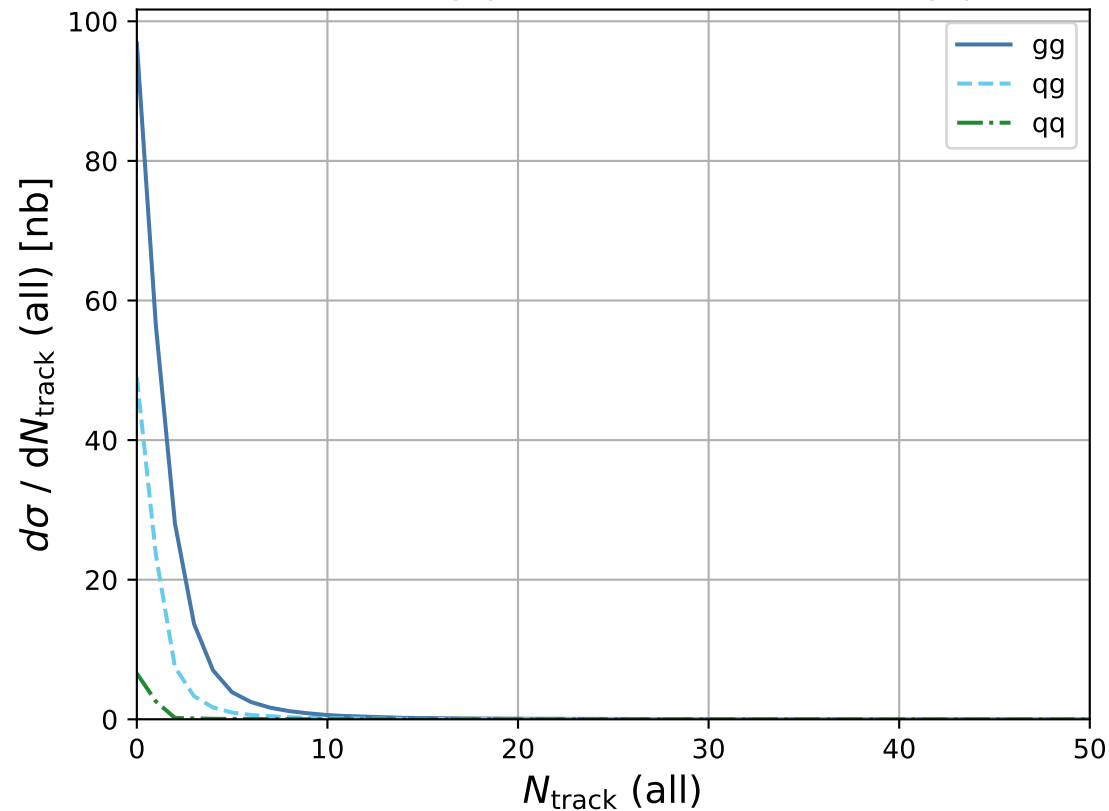

Supplement: Supplementary file 2 [file LHC_additional_plots.pdf]
